# Supplementary material for: Wasserstein Dictionaries of Persistence Diagrams
Source: arXiv:2304.14852 source file (2023-09-15)
Supplement: Supplementary file 1 [file commands.tex]

\newcommand{\Ens}{\mathcal{E}}
\newcommand{\Dict}{\mathcal{D}}
\newcommand{\Diag}{\mathcal{X}}
\newcommand{\Lamb}{\bm{\lambda}}
\newcommand{\Bary}{\julienRevision{Y}(\Lamb , \Dict)}
\newcommand{\BaryAll}{\julienRevision{Y}(\Lamb_{n} , \Dict)}
\newcommand{\BaryGen}{\julienRevision{Y}(\Lamb^{*} , \Dict_{*})}
\newcommand{\BaryGenAll}{\julienRevision{Y}(\Lamb_{n}^{*} , \Dict_{*})}
\newcommand{\BaryLamb}{\julienRevision{Y}(\Lamb)}
\newcommand{\BaryLambO}{\julienRevision{Y}(\Lamb^{t})}
\newcommand{\BaryDict}{\julienRevision{Y}(\Dict)}
\newcommand{\BaryDictO}{\julienRevision{Y}(\Dict_{t})}
% \newcommand{\Bary}{B_2(\Lamb , \Dict)}
% \newcommand{\BaryAll}{B_2(\Lamb_{n} , \Dict)}
% \newcommand{\BaryGen}{B_2(\Lamb^{*} , \Dict_{*})}
% \newcommand{\BaryGenAll}{B_2(\Lamb_{n}^{*} , \Dict_{*})}
% \newcommand{\BaryLamb}{B_2(\Lamb)}
% \newcommand{\BaryLambO}{B_2(\Lamb^{t})}
% \newcommand{\BaryDict}{B_{2}(\Dict)}
% \newcommand{\BaryDictO}{B_{2}(\Dict_{t})}
\newcommand{\wasserstein}{\julienRevision{W}}
\newcommand{\War}{\wasserstein^2}
\newcommand{\Ass}{\phi_{1}}
\newcommand{\AssM}{\phi_{m}}
\newcommand{\AssI}{\phi_{i}}


\newcommand{\keanu}[1]{\textcolor{black}{#1}}

\newcommand{\frechetEnergy}{E_F}
\newcommand{\dictionaryEnergy}{E_D}
\newcommand{\weightEnergy}{E_W}
\newcommand{\atomEnergy}{E_A}
\newcommand{\individualAtomEnergy}{e_A}


\newcommand{\julien}[1]{\textcolor{black}{#1}}
% uncomment the line below to disable color
% \renewcommand{\julien}[1]{\textcolor{blue}{#1}}
\newcommand{\julienQuestion}[1]{\textcolor{black}{#1}}
% uncomment the line below to disable color
% \renewcommand{\julienQuestion}[1]{\textcolor{blue}{#1}}

\newcommand{\toDiscuss}[1]{\textcolor{red}{#1}}

\newcommand{\toAddress}[1]{\textcolor{purple}{#1}}

\newcommand{\julienRevision}[1]{\textcolor{black}{#1}}

\renewcommand{\figureautorefname}{Fig.}
\renewcommand{\sectionautorefname}{Sec.}
\renewcommand{\subsectionautorefname}{Sec.}
\renewcommand{\equationautorefname}{Eq.}
\renewcommand{\tableautorefname}{Tab.}
\renewcommand{\algorithmautorefname}{Alg.}
\newcommand{\lineautorefname}{Alg.}
